# Supplementary material for: MathQA: Towards Interpretable Math Word Problem Solving with Operation-Based Formalisms
Source: arXiv:1905.13319 source file (2019-05-30)
Supplement: Supplementary file 1 [file appendix.tex]

\appendix
\section{Appendices}

\label{sec:appendix}

\subsection{Automatic  Annotation using Rationales}
%The first strategy is to leverage annotated rationales in the \aqua\ dataset to align problems to operation programs. 
 Our automatic annotation strategy focuses on problems with rationales that are mostly accurate in their description of the problem solving process. Given a word problem x, we expect that a number mentioned in the rationale for x is important to forming a corresponding operation program. In other words, we assume that each number in the rationale either directly appears in an operation program associated with x or can be calculated from previously mentioned numbers using operations in the program. 

%The intuition behind our automatic annotation is that an operation program can be generated for a specific problem by trying to derive numbers mentioned in the rationales. Some numbers in the rationale may be ignored, as long as the induced program leads to the correct final solution. \aida{The following is not correct. even if we cannot get to the number within a rationale we might still be able to get to the final number, so as the known number we keep the numbers in the rationale which we can actually reinstruct at least one program for}

% In general the final is calculated after k of calculations(k-th level of indirection). However by keeping all the numbers that are already searched, the next number mentioned in rationale should be calculable with 0 or 1 level of indirection(0-th level of indirection means that we already have the number.) 

We design an algorithm that uses these assumptions to generate feasible operation programs from \aqua\ rationales. Our automatic annotation algorithm uses a dynamic programming approach to derive operation programs from the numbers in the rationale. Operations are selected sequentially. Some numbers in the rationale may be ignored, as long as the induced program leads to the correct final solution. 

The algorithm takes in the numbers appearing in the problem, domain-specific constants and numbers calculated at previous timesteps as input. At each time step (t) we only search for combinations of operations and arguments that can result in the  $t^{th}$ number mentioned in the rationale. This process continues until the final answer is reached.

%leverage numbers in rationales to form operation programs (Sketched in Algorithm~\ref{alg:dyn}) \aida{should I modify the algorithm?}. The inputs are the numbers in the problem, the rationale text, and the correct final answer, and the output is the list of acceptable programs. 
%\hanna{I am still not sure about this} Given numbers in the problem, defined constant and numbers calculated in previous time steps, at each time step (t) we only search for combinations of operations and arguments that can result in the  $t^{th}$ number mentioned in the rationale. and we continue this process until the final answer is reached. \hanna{Is this correct?} \aida{yes.} \hanna{Explain this with one example; basically explain your dynamic programming step with one example, Something like this: In this problem, the number xxx from the rationale can be derived from operation aaaa and operation bbbb using other numbers.  } 
We keep the plausible paths that show how numbers in rationales are reproduced. We use the mathematical expressions described in the rationales to prune programs which do not use those expressions. Finally, we prune those paths that do not achieve the correct solution. We use automatic annotations for problems which lead to at most five operation programs.

Similar as the previous setup, we employ human annotators to validate automatically-annotated operation programs. The annotators check whether the  problems and annotated programs are aligned or not. Due to the noise in the rationales, only $80.39\%$ of those problems pass our human validation. This is mainly due to the fact that the rationales are not complete programs and fail to explicitly describe all important numbers and operations required to solve the problem.

 \begin{figure*}
\centering
  \includegraphics[width=.5\textwidth]{validation_img.pdf}
 \caption{Tracking of agreement among crowdsourcing workers on validation task}
    \label{fig:bar-chart}
\end{figure*}

 \begin{figure*}[t]
\centering.
  \includegraphics[width=1\textwidth]{Data_collection.pdf}
 \caption{Complete pipeline of Data Collection}
    \label{fig:pipeline}
\end{figure*}
\section{Supplemental Material}

\begin{figure}
\centering
  \includegraphics[width=.5\textwidth]{plot.pdf}
 \caption{Solvability of Original AQuA dataset (in addition to these unsolvable problems, 35 problems in the train set did not contain words)}
    \label{fig:bar-chart}
\end{figure}

\begin{table}[h]
\begin{tabular}{  l | l } 
Major Categories  & Count \\ \hline
General & 34990\\
Physics  & 10260 \\
Probability  & 7338 \\
Geometry & 2661       \\ 
Gain-Loss  & 7178\\
Other & 35040\\
\end{tabular}
\caption{Domain Category Distribution for Train Set}
\end{table}

\begin{table}[h]
\begin{tabular}{  l | l | l  } 
Split  & Geometry & Physics    \\ \hline
Train & ? & ?       \\ 
Validation  & ? & ?  \\
Test  & ? & ? \\ \hline
Total & 6500 & 2500\\
\end{tabular}
\caption{Our dataset}
\end{table}

\begin{figure}[]
\centering
  \includegraphics[width=.5\textwidth]{chart.png}
 \caption{Distributions for length of programs among problems}
    \label{fig:bar-chart}
\end{figure}

\begin{table}[h]
\begin{tabular}{  l | l  } 
Category   & Average Number of Operations \\ \hline
General & 5.3111 \\ 
Physics & 5.0113 \\ 
Probability & 5.4417 \\ 
Geometry &  4.7850  \\ 
Gain-Loss  & 6.0848\\
Other &  4.8260 \\ \hline
Total  & 5.2005   \\
\end{tabular}
\caption{Total number of operations by categories}
\label{my-label2}
\end{table}

\begin{table}[h]
\resizebox{\columnwidth}{!}{%
\begin{tabular}{  l | l | l | 1 |  1  } 
Category  & #Annotated & #Validated & F1  & #Expanded   \\ \hline
Geometry  & 2194 & 1816 & 82.7711 & 3035  \\ 
Physics & 2287 & 2211 & 96.6768 & 8136 \\
Probability  & 689 & 655 & 95.0653 & 3757  \\
Gain-Loss  & 946 & 916 & 96.8287 & 4213 \\ 
General  & 3130 & 3056 &97.6357 & 17499 \\ 
Other  & 643 & 636 & 98.9113 & 1555 \\ \hline
All & & & & \\ \\
\end{tabular}
}
\caption{Annotation Statistics}
\label{my-label2}
\end{table}

\begin{table}[h]
\caption{Dataset Statistics}
\resizebox{\columnwidth}{!}{%
\begin{tabular}{  l | l | l | l | 1 | 1 } 
Category  & Total &  Ave. Prob Words & Ave. Prob Sent & #Vocab  & Ave ops length   \\ \hline
Geometry  & 3035 & 35.1023 & 2.0675 & 1818 &  4.7850  \\ 
Physics & 8136 & 40.0725 & 2.4103 & 2860 & 5.0113 \\
Probability  & 3757  & 34.7340 & 2.1737 & 1778 &  5.4417  \\
Gain-Loss  &  4213 & 36.1217 & 2.8446 & 1502 &  6.0848 \\ 
General  & 17499 & 37.7049 & 2.2584 & 4218 & 5.3111 \\ 
Other  &  1555 & 35.0044 & 2.3674 &  1393 & 4.8260 \\ \hline
All & & & 2.34983 & 6664 &  \\
\end{tabular}
}
\caption{AQUA-Prog src and target size and Vocabulary cound.}
\label{my-label2}
\end{table}
\label{sec:supplemental}

\begin{figure*}[t]
\centering
  \includegraphics[width=1\textwidth]{figure_eight_smal.png}
 \caption{A View of our human in the loop annotation task. Since the operations in future steps might be dependant to the result of this step, after each calculation the result is added to the stack of possible arguments.(b). Submission is only possible when they reach to close range of correct answer and we log their solution pattern in operation formula field.(c)}
    \label{fig:categorization}
\end{figure*}
\begin{figure*}[t]
\centering
  \includegraphics[width=1\textwidth]{validation_task.png}
 \caption{A View of our human validation task. Two separate annotations are found for a problem where both result in correct values. But the one on the right is logically wrong and should be mark as invalid.}
    \label{fig:categorization}
\end{figure*}
